# Supplementary material for: A Bayesian Optimal Phase II Design for Randomized Immunotherapy Trials with Delayed Treatment Effects
Source: arXiv:2509.00238 ancillary file (2025-08-29)
Supplement: Supplementary file 1 [file Supplementary.pdf]

# Supplementary Material for "A Bayesian Optimal Phase II Design for Randomized Immunotherapy Trials with Delayed Treatment Effects"

Zhongheng Cai and Haitao Pan \*

Department of Biostatistics, St. Jude Children's Research Hospital,  
Memphis, USA

## 1 When There is an Early Stopping Probability

Recall that in Section 3 (Real Data Example), the following settings are used:

- Sample size for the two-stage design: 28 (interim), 40 (final)
- Best-guess for  $S$ :  $S_{\text{likely}} = 2.28$
- Accrual rate: 6 patients per arm per month; follow-up duration: 6 months
- Prior for  $S$ :  $\text{Gamma}(12.86, 0.19) \cdot I(2, 2.5)$

Under these assumptions, the probability of early stopping under  $H_0$  is 0.2957 and 0.2379 when the true but unknown  $S$  equals 2 and 2.5, respectively.

Some practitioners may find these early stopping probabilities insufficiently high. Suppose we instead require the early stopping probability (PS) to be no less than 0.4. To accommodate this, we recalculated the interim and final sample sizes using the function `Two_stage_sample_size(.)` with the parameter `earlystop_prob = 0.4`, while keeping other parameters unchanged and fixing  $S_{\text{likely}} = 2.28$ . This ensures that the probability of early stopping reaches at least 0.4 for  $S \in [L, U]$ . The R code is demonstrated as below:

---

\*Corresponding author: Haitao.Pan@stjude.org

```

> earlystop_prob = 0.4
> Two_stage_sample_size(median.1 = median.1, median.2 = median.2,
  L = L, U = U, S_likely = S_likely, err1 = err1, err2 = err2,
  trunc.para = trunc.para, FUP = FUP, rate = rate,
  earlystop_prob = earlystop_prob, seed = 123)
#> $sample_size
#> [1] 39 52
#> $optimal
#> [1] 0.9500 1.0000 0.0764 0.9247

```

According to the results, the required two-stage sample sizes to meet the early stopping threshold of 0.4 are 39 for interim analysis and 52 for the final analysis. Based on these sample sizes, we further evaluate performance metrics for a range of true  $S$  values, specifically  $S = 2.0, 2.1, 2.2, 2.3, 2.4, 2.5$ , which are summarized in the Table 1.

Table 1: Percentage of rejecting the null (PRN), percentage of early termination (PET), the actual sample size (each arm), and trial duration under the DTE-BOP2 design with true  $S = 2, 2.1, 2.2, 2.3, 2.4, 2.5$  for two-stage sample size (39, 52) per arm.

|           |             | PRN (%) | PET (%) | Sample size | Trial duration <sup>a</sup> |
|-----------|-------------|---------|---------|-------------|-----------------------------|
| $S = 2$   | $H_0$ holds | 7.4     | 44.9    | 46.2        | 11.1                        |
|           | $H_1$ holds | 93.7    | 4.6     | 51.4        | 14.3                        |
| $S = 2.1$ | $H_0$ holds | 7.5     | 44.2    | 46.3        | 11.1                        |
|           | $H_1$ holds | 93.0    | 5.0     | 51.4        | 14.3                        |
| $S = 2.2$ | $H_0$ holds | 7.8     | 43.7    | 46.3        | 11.2                        |
|           | $H_1$ holds | 92.5    | 5.2     | 51.3        | 14.3                        |
| $S = 2.3$ | $H_0$ holds | 7.7     | 42.8    | 46.4        | 11.2                        |
|           | $H_1$ holds | 91.9    | 5.7     | 51.3        | 14.2                        |
| $S = 2.4$ | $H_0$ holds | 7.7     | 42.1    | 46.5        | 11.3                        |
|           | $H_1$ holds | 91.7    | 5.8     | 51.2        | 14.2                        |
| $S = 2.5$ | $H_0$ holds | 8.0     | 41.2    | 46.6        | 11.4                        |
|           | $H_1$ holds | 91.2    | 6.1     | 51.2        | 14.2                        |

<sup>a</sup> In months.

The results presented in Table 1 show that increasing the two-stage sample size from (28, 40) to (39, 52) successfully raises the early stopping probability under  $H_0$  above the pre-specified threshold of 0.4 for all considered values of  $S \in [2.0, 2.5]$ . Specifically, PET under  $H_0$  ranges from 41.2% to 44.9%, compared to the original range of 23.8% to 29.6% with

smaller sample sizes. This represents an approximate 15–20 percentage point increase in early stopping probability, achieved at the cost of an enlarged sample size. Such a shift aligns with intuition: by increasing the interim sample size, the design accumulates more information at the first stage, thereby improving the chance of detecting lack of efficacy early under  $H_0$ . Notably, this adjustment allows the trial to more reliably stop early when the treatment is ineffective, which is desirable from both ethical and resource-efficiency perspectives. At the same time, under  $H_1$ , the early stopping probability remains low (ranging from 4.6% to 6.1%), ensuring a low risk of erroneously terminating a truly effective treatment. Power remains above 91% across all values of  $S$ , and the average sample size under  $H_1$  increases modestly to around 51 patients per arm. These results confirm that increasing the sample size improves early stopping properties under the null while preserving strong performance under the alternative.

## 2 Sensitivity Analysis

### 2.1 Performance in a Three-Stage Design

While the primary design considered in this manuscript is a two-stage adaptive trial, we now explore the extension of our method to a multi-stage setting by evaluating a three-stage design. Although a closed-form solution for optimal sample sizes in the three-stage design is not available, we assess whether the interim and final sample sizes derived from the two-stage setting provide robust performance when an additional interim analysis is incorporated.

Specifically, we set the interim analysis points at `n.interim = (13, 28, 40)` and use the function `get.optimal_2arm_pieewise(.)` to determine the optimal decision boundaries. The R code and resulting values are shown below:

```
> n.interim = c(13, 28, 40)
> get.optimal_2arm_pieewise(median.1 = median.1, median.2 = median.2,
  L = L, U = U, S_likely = 2.28, Uniform = FALSE,
  trunc.para = c(12.86, 0.19), err1 = 0.1, n.interim = n.interim,
  rate = rate, FUP = FUP, track = TRUE, nsim = 10000,
  control = TRUE, control.point = c(L, U))
#> $optimal
#> [1] 0.9500 1.0000 0.0875 0.8678
```

The resulting optimal values for  $\lambda$  and  $\gamma$  are 0.95 and 1.00, respectively. To evaluate the designs performance, we examine key operating characteristics under a range of true  $S$  values:  $S = 2.0, 2.1, 2.2, 2.3, 2.4, 2.5$ . The results are summarized in Table 2.

Compared to the original two-stage design, the three-stage design yields similar performance in terms of power, Type I error, and average sample size. Notably, the probability of early stopping under  $H_0$  increases slightly, indicating that the additional interim analysis

offers more opportunities to terminate trials early when the treatment is ineffective. This suggests that the inclusion of a third stage can improve efficiency without compromising the designs overall statistical properties. However, the three-stage design also introduces additional logistical and operational complexity. Each interim analysis requires data cleaning, statistical review, and potentially Data Monitoring Committee (DMC) involvement, all of which increase administrative burden and may delay trial progression. Furthermore, repeated interim analyses may raise concerns about information leakage or operational bias, particularly in unblinded settings. These practical considerations should be weighed against the marginal statistical gains when deciding whether to adopt a multi-stage design in real-world applications.

Table 2: Percentage of rejecting the null (PRN), percentage of early termination (PET), the actual sample size (each arm), and trial duration under the DTE-BOP2 design with true  $S = 2, 2.1, 2.2, 2.3, 2.4, 2.5$  for three-stage design.

|           |             | PRN (%) | PET (%) | Sample size | Trial duration <sup>a</sup> |
|-----------|-------------|---------|---------|-------------|-----------------------------|
| $S = 2$   | $H_0$ holds | 8.3     | 28.6    | 36.5        | 10.4                        |
|           | $H_1$ holds | 88.5    | 7.0     | 39.1        | 12.1                        |
| $S = 2.1$ | $H_0$ holds | 8.4     | 27.8    | 36.6        | 10.5                        |
|           | $H_1$ holds | 87.8    | 7.5     | 39.1        | 12.1                        |
| $S = 2.2$ | $H_0$ holds | 8.4     | 26.9    | 36.7        | 10.6                        |
|           | $H_1$ holds | 87.0    | 7.4     | 39.1        | 12.1                        |
| $S = 2.3$ | $H_0$ holds | 8.2     | 26.1    | 36.8        | 10.6                        |
|           | $H_1$ holds | 86.6    | 7.5     | 39.1        | 12.1                        |
| $S = 2.4$ | $H_0$ holds | 8.3     | 25.1    | 36.9        | 10.7                        |
|           | $H_1$ holds | 85.8    | 7.6     | 39.1        | 12.1                        |
| $S = 2.5$ | $H_0$ holds | 8.3     | 24.0    | 37.1        | 10.8                        |
|           | $H_1$ holds | 85.9    | 7.3     | 39.1        | 12.1                        |

<sup>a</sup> In months.

## 2.2 Sensitivity to Different Priors for $S$

To assess the robustness of the proposed design to the prior specification for the parameter  $S$ , we conduct a sensitivity analysis under two alternative scenarios:

1. An expert-elicited prior with high concentration around the believed value of  $S$ .

2. A vague default prior,  $S \sim \text{Gamma}(1, 1) \cdot I(L, U)$ .

In the first scenario, we incorporate prior information provided by three hypothetical domain experts:

- Expert A: Believes the mean of  $S$  is 2.28.
- Expert B: Believes the median of  $S$  is 2.4.
- Expert C: Believes the mean is 2.4 and the median is 2.3.

These inputs are combined using the `trunc_gamma_para(.)` function to fit a truncated Gamma distribution over the plausible range  $S \in [2, 2.5]$ . The following R code demonstrates the procedure and the resulting hyperparameters:

```
expert_data_correct <- list(
  list(mean = 2.28, median = NULL, sd = NULL, q25 = NULL, q975 = NULL),
  list(mean = NULL, median = 2.4, sd = NULL, q25 = NULL, q975 = NULL),
  list(mean = 2.4, median = 2.3, sd = NULL, q25 = NULL, q975 = NULL)
)

param_1 <- trunc_gamma_para(
  L = 2,
  U = 2.5,
  expert_data = expert_data_correct,
  weights = c(4, 4, 2, 1, 1),
  num_cores = 4
)

print(param_1)
#> $shape
#> [1] 19.48974
#>
#> $scale
#> [1] 0.2736842
```

Figure 2 displays the resulting prior density for  $S$ , which is notably more concentrated around 2.42 compared to the prior used in the main analysis ( $S \sim \text{Gamma}(12.86, 0.19) \cdot I(2, 2.5)$ ).

Using this updated prior and setting  $S_{\text{likely}} = 2.28$ , we re-derive the optimal tuning parameters for the design. The optimal values of  $\lambda$  and  $\gamma$  remain unchanged at 0.95 and 1.00, respectively. Table 3 summarizes the corresponding operating characteristics across a range of true  $S$  values.

The results indicate that the use of a more informative prior does not significantly affect the key performance metrics of the design. Both type I error and power remain stable and consistent with those observed under the default prior specification. This suggests that the design is robust to moderate changes in prior assumptions for  $S$ , reinforcing its practical applicability.

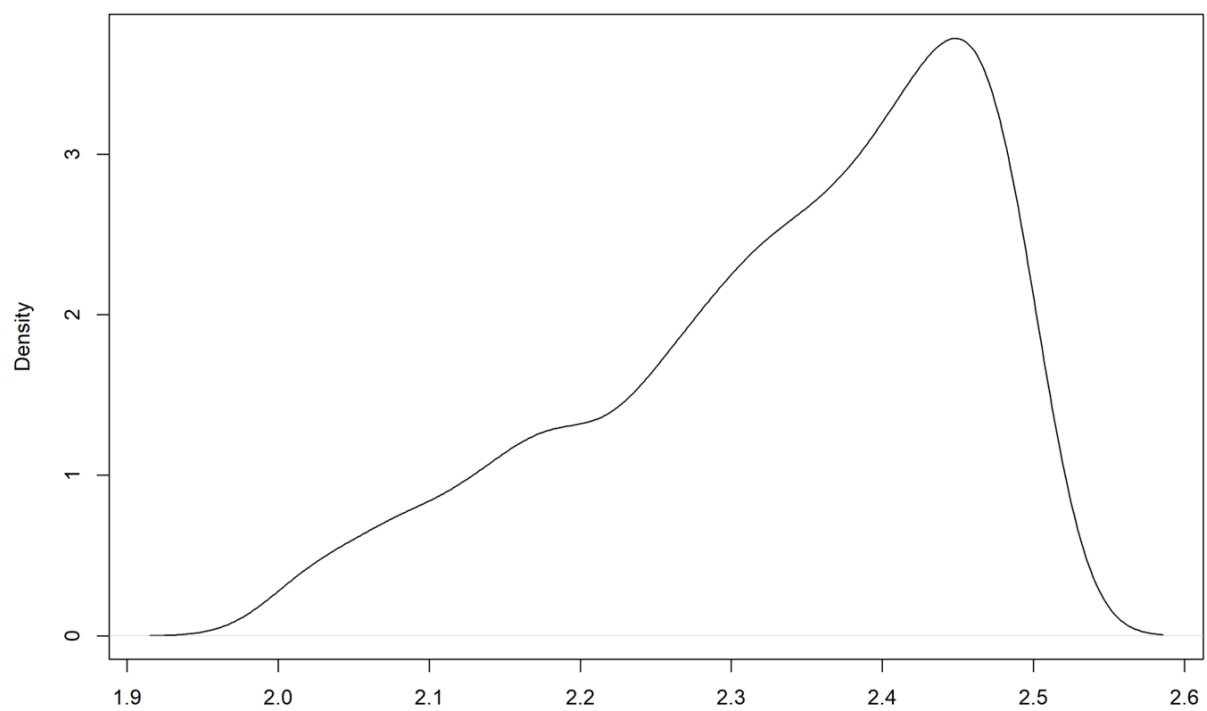

Figure 1: Density plot of the expert-elicited prior  $S \sim \text{Gamma}(19.49, 0.27) \cdot I(2, 2.5)$

Table 3: Percentage of rejecting the null (PRN), percentage of early termination (PET), the actual sample size (each arm), and trial duration under the DTE-BOP2 design with true  $S = 2, 2.1, 2.2, 2.3, 2.4, 2.5$  for prior  $S \sim \text{Gamma}(19.49, 0.27)I(2, 2.5)$ .

|           |             | PRN (%) | PET (%) | Sample size | Trial duration <sup>a</sup> |
|-----------|-------------|---------|---------|-------------|-----------------------------|
| $S = 2$   | $H_0$ holds | 8.3     | 28.5    | 36.6        | 10.4                        |
|           | $H_1$ holds | 88.6    | 6.9     | 39.2        | 12.1                        |
| $S = 2.1$ | $H_0$ holds | 8.4     | 27.8    | 36.7        | 10.5                        |
|           | $H_1$ holds | 87.8    | 7.3     | 39.1        | 12.1                        |
| $S = 2.2$ | $H_0$ holds | 8.4     | 26.8    | 36.8        | 10.6                        |
|           | $H_1$ holds | 87.1    | 7.3     | 39.1        | 12.1                        |
| $S = 2.3$ | $H_0$ holds | 8.2     | 26.1    | 36.9        | 10.6                        |
|           | $H_1$ holds | 86.7    | 7.4     | 39.1        | 12.1                        |
| $S = 2.4$ | $H_0$ holds | 8.3     | 25.1    | 37.0        | 10.7                        |
|           | $H_1$ holds | 85.9    | 7.5     | 39.1        | 12.1                        |
| $S = 2.5$ | $H_0$ holds | 8.3     | 23.9    | 37.1        | 10.8                        |
|           | $H_1$ holds | 86.1    | 7.2     | 39.1        | 12.1                        |

<sup>a</sup> In months.

If sufficient prior information is unavailable to specify the hyperparameters  $s_1$  and  $s_2$  for the distribution of  $S$ , we recommend adopting a default prior with  $s_1 = 1$  and  $s_2 = 1$ . This choice corresponds to a  $\text{Gamma}(1, 1)$  prior truncated to the interval  $[L, U]$ , which yields a near-uniform distribution over the plausible range of  $S$ , reflecting minimal prior information. The density plot can be seen in Figure 2.

Using this vague prior and setting  $S_{\text{likely}} = 2.28$ , the optimal tuning parameters for the design are re-estimated. As shown below, the resulting values of  $\lambda$  and  $\gamma$  remain unchanged at 0.95 and 1.00, respectively. We also find that (not shown here) the average type I error and power are also comparable to those obtained under both the expert-elicited prior and the prior used in the main analysis.

```
#> $optimal
#> [1] 0.9500 1.0000 0.0876 0.8694
```

Overall, the results demonstrate that the DTE-BOP2 design is robust to the choice of prior for  $S$ . The key operating characteristics—including optimal tuning parameters  $(\lambda, \gamma)$ , average type I error, average power, and early stopping behavior—remain stable under both informative and vague prior specifications. This robustness enhances the practical appeal of the method, particularly in scenarios where eliciting reliable prior information is challenging.

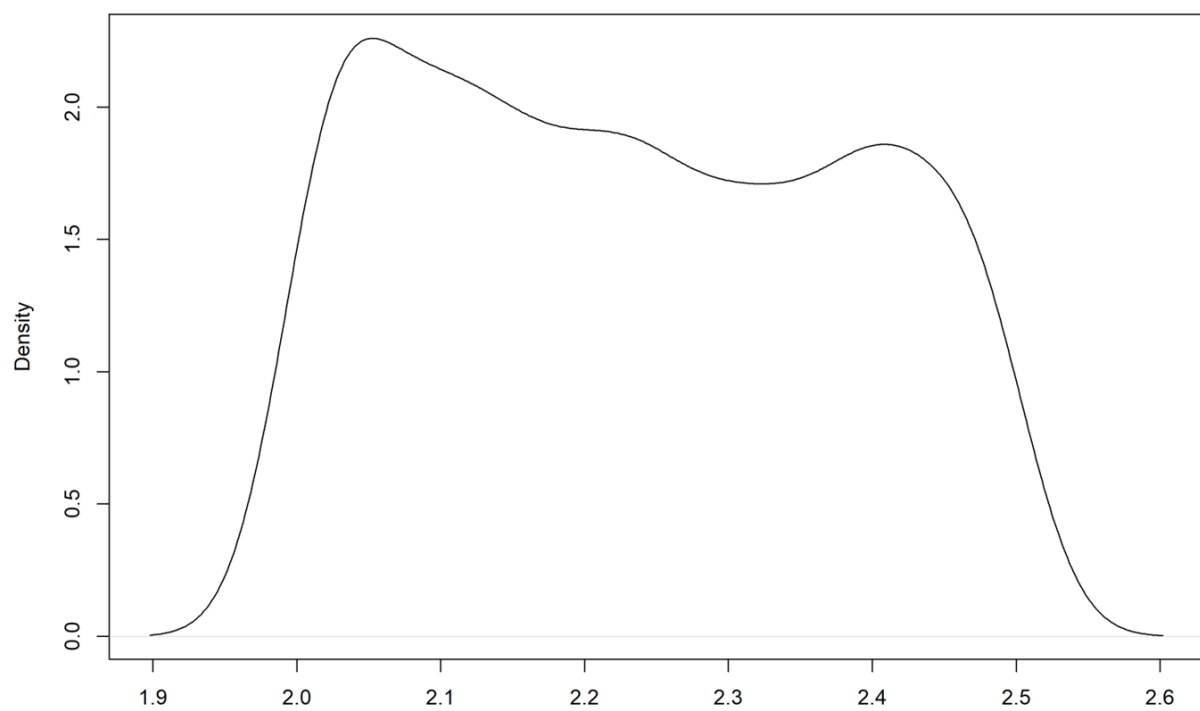

Figure 2: Density plot of  $S$  under the default prior  $(\text{Gamma}(1, 1) \cdot I(L, U))$



### 3 On Slow and Fast Recruitment Rate

In the main analysis, we assume a recruitment rate of 6 patients per arm per month. To assess the sensitivity of the design to accrual speed, we additionally consider alternative scenarios with slower and faster recruitment rates, specifically 3, 9, and 12 patients per arm per month.

Table 4: Early stopping rate under  $H_0$ , early stopping rate under  $H_1$ , Type I error, power, average sample size under  $H_1$ , and trial duration under  $H_1$  for different accrual rate.

| Scenario  |           | PET(%)( $H_0$ ) | PET(%)( $H_1$ ) | Type I Error(%) | Power(%) | Average Sample Size ( $H_1$ ) | Duration <sup>a</sup> ( $H_1$ ) |
|-----------|-----------|-----------------|-----------------|-----------------|----------|-------------------------------|---------------------------------|
| rate = 3  | $S = 2$   | 40.9            | 3.1             | 8.2             | 93.6     | 39.6                          | 19.0                            |
|           | $S = 2.1$ | 39.8            | 3.3             | 8.4             | 92.8     | 39.6                          | 19.0                            |
|           | $S = 2.2$ | 39.9            | 3.5             | 8.5             | 92.5     | 39.6                          | 18.9                            |
|           | $S = 2.3$ | 39.5            | 3.8             | 8.8             | 91.9     | 39.5                          | 19.0                            |
|           | $S = 2.4$ | 38.9            | 3.6             | 8.7             | 91.9     | 39.6                          | 18.9                            |
|           | $S = 2.5$ | 38.3            | 3.9             | 8.5             | 91.1     | 39.5                          | 18.9                            |
| rate = 6  | $S = 2$   | 29.6            | 7.1             | 8.4             | 88.0     | 39.1                          | 12.1                            |
|           | $S = 2.1$ | 28.3            | 7.4             | 8.9             | 87.2     | 39.1                          | 12.1                            |
|           | $S = 2.2$ | 27.1            | 7.1             | 8.7             | 87.1     | 39.1                          | 12.1                            |
|           | $S = 2.3$ | 26.3            | 7.1             | 8.7             | 86.6     | 39.1                          | 12.1                            |
|           | $S = 2.4$ | 25.0            | 7.3             | 8.8             | 86.2     | 39.1                          | 12.1                            |
|           | $S = 2.5$ | 23.8            | 7.6             | 8.7             | 85.5     | 39.1                          | 12.1                            |
| rate = 9  | $S = 2$   | 19.4            | 9.4             | 8.6             | 84.9     | 38.9                          | 9.8                             |
|           | $S = 2.1$ | 18.2            | 9.2             | 8.8             | 84.7     | 38.9                          | 9.8                             |
|           | $S = 2.2$ | 17.2            | 9.3             | 8.9             | 83.9     | 38.9                          | 9.8                             |
|           | $S = 2.3$ | 15.9            | 9.2             | 8.8             | 83.4     | 38.9                          | 9.8                             |
|           | $S = 2.4$ | 15.0            | 9.3             | 8.8             | 82.7     | 38.9                          | 9.8                             |
|           | $S = 2.5$ | 13.9            | 8.9             | 8.7             | 82.7     | 38.9                          | 9.8                             |
| rate = 12 | $S = 2$   | 14.0            | 10.5            | 8.9             | 82.8     | 38.7                          | 8.4                             |
|           | $S = 2.1$ | 13.3            | 10.9            | 9.1             | 82.1     | 38.7                          | 8.6                             |
|           | $S = 2.2$ | 12.6            | 10.7            | 9.1             | 81.6     | 38.7                          | 8.6                             |
|           | $S = 2.3$ | 11.9            | 10.7            | 9.3             | 81.4     | 38.7                          | 8.6                             |
|           | $S = 2.4$ | 11.7            | 10.7            | 9.1             | 80.6     | 38.7                          | 8.6                             |
|           | $S = 2.5$ | 11.5            | 10.7            | 9.3             | 79.8     | 38.7                          | 8.6                             |

<sup>a</sup> In months.

Table 4 summarizes the impact of varying recruitment rates (3, 6, 9, and 12 patients per arm per month) on key operating characteristics of the proposed design, including early stopping probability under  $H_0$  (PET( $H_0$ )) and  $H_1$  (PET( $H_1$ )), type I error, power, average sample size, and trial duration under  $H_1$ . As expected, increasing the recruitment rate leads to a reduction in early stopping probability under  $H_0$ . For instance, when  $S = 2$ , PET( $H_0$ ) decreases from 40.9% at rate = 3 to 14.0% at rate = 12. This is because faster accrual reduces the amount of follow-up information available at interim analyses, thereby limiting the opportunity to terminate early for futility.

Importantly, the type I error remains relatively stable across all accrual rates and values of  $S$ , consistently staying within the range of 8.2% to 9.3%, suggesting that the design preserves its frequentist error control under various accrual conditions. However, power shows a clear downward trend as the recruitment rate increases. For example, for  $S = 2.5$ , the power drops from 91.1% at rate = 3 to 85.5% at rate = 6, 82.7% at rate = 9, and further to 79.8% at rate = 12. Even when comparing with the base scenario at rate = 6 (used in the main analysis), the power declines by

approximately 3% at rate = 9 and 6% at rate = 12 across comparable values of  $S$ . This decline occurs because faster accrual allows less time for delayed treatment effects to emerge before interim or final decision-making, which can dilute the observed treatment benefit. Average sample size under  $H_1$  remains approximately 39 across all rates, as the stopping rule is driven by posterior probabilities rather than accrual speed. Meanwhile, the total trial duration under  $H_1$  decreases substantially with faster recruitment—from approximately 19 months at rate = 3 to just under 9 months at rate = 12—highlighting the trade-off between operational efficiency and statistical performance when setting accrual targets.

Another important observation is that the gap between  $\text{PET}(H_0)$  and  $\text{PET}(H_1)$  narrows substantially as the recruitment rate increases. At an accrual rate of 3 patients per arm per month, the difference in early stopping probability between  $H_0$  and  $H_1$  can exceed 35%; however, this difference shrinks to less than 4% when the rate increases to 12. This convergence suggests that early stopping becomes less discriminative under fast accrual: when early termination occurs, it is no longer clear whether it reflects a true lack of efficacy (appropriate under  $H_0$ ) or a premature decision that fails to capture a delayed treatment benefit (problematic under  $H_1$ ). This pattern is consistent with the assumed delayed treatment effect, wherein the treatment and control arms exhibit similar event patterns in the early part of the study. Under rapid accrual, many patients may not be followed long enough for the treatment effect to manifest before interim decisions are made. As a result, early stopping decisions become increasingly based on incomplete information, reducing their ability to differentiate between effective and ineffective treatments (Liu et al. 2025, Horiguchi et al. 2019).

## 4 Varying $S_{\text{likely}}$

To evaluate the robustness of the proposed design to the specification of the best-guessed separation time point, we conduct a sensitivity analysis by varying  $S_{\text{likely}}$  from 2.0 to 2.5 in increments of 0.1. In all scenarios, we fix the overall median survival times for the control and treatment arms as  $\bar{\mu}_0 = 2.8$  and  $\bar{\mu}_1 = 3.5$ , respectively. Given that the median survival times before and after the separation point, denoted as  $\tilde{\mu}_0$  and  $\tilde{\mu}_1$ , are functions of  $S_{\text{likely}}$ , they are recalculated accordingly in each scenario.

We use the original sample size of (28, 40) per arm, which was determined under  $S_{\text{likely}} = 2.28$ , and evaluate the designs operating characteristics across the range of  $S_{\text{likely}}$ . For the true but unknown  $S$ , we consider two representative values:  $S = 2.0$  and  $S = 2.5$ . The type I error and power under each scenario are summarized in Table 5.

The results indicate that type I error is well-controlled (below 0.10) across all examined values of  $S_{\text{likely}}$ . However, when smaller values of  $S_{\text{likely}}$  are specified during the design stage (e.g.,  $S_{\text{likely}} = 2.0, 2.1, 2.2$ ), the power drops below 0.85. This observation is expected, as the original design was calibrated at  $S_{\text{likely}} = 2.28$ , yielding pre- and post-separation medians of  $\tilde{\mu}_0 = 2.8$  and  $\tilde{\mu}_1 = 6.57$ . In contrast, setting  $S_{\text{likely}} = 2.0$  leads to a smaller post-separation median of  $\tilde{\mu}_1 = 5.25$ , which dilutes the contrast between arms and reduces power. In contrast, when larger values of  $S_{\text{likely}}$  are used (e.g.,  $S_{\text{likely}} = 2.3, 2.4, 2.5$ ), power consistently remains above 0.85.

To ensure that the power remains above 85% regardless of the true value of  $S$  and the prespecified  $S_{\text{likely}}$  within  $[2.0, 2.5]$ , we recalculated the required sample size using a conservative choice of  $S_{\text{likely}} = 2.0$ . The corresponding R code and output are provided below:

```
> median.1 = 2.8
> median.2 = 3.5
> L = 2
> U = 2.5
> S_likely = 2
> trunc.para = c(12.86, 0.19)
> rate = 6
> FUP = 6
> err1 = 0.1
> err2 = 0.15
> Two_stage_sample_size(median.1 = median.1, median.2 = median.2,
  L = L, U = U, S_likely = S_likely, err1 = err1, err2 = err2,
  trunc.para = trunc.para, FUP = FUP, rate = rate,
  weight = 0.5, earlystop_prob = NULL)
#> $sample_size
#> [1] 44 63
#> $optimal
#> [1] 0.9500 1.0000 0.0813 0.8786
```

The updated interim and final sample sizes are 44 and 63 per arm, respectively. Using this revised design, we re-evaluate the operating characteristics across combinations of true  $S$  and assumed  $S_{\text{likely}}$ , as reported in Table 6.

Based on the results, we summarize the following key findings:

1. With a maximum sample size of 63 per arm, the design achieves type I error control at the 0.1 level and maintains power above 0.85 across all combinations of the true separation time  $S$  and the user-specified best-guess  $S_{\text{likely}}$ . This demonstrates a form of *doubly robustness*—the design is robust to both the true (but unknown) separation time  $S$  and the elicited best-guess value  $S_{\text{likely}}$ , provided that both lie within the prespecified interval  $[L, U]$  and a conservative choice of  $S_{\text{likely}}$  (e.g., the lower bound  $L$ ) is used during the design stage.
2. A larger upper bound  $U$  increases the required sample size, since the design must maintain power above  $1 - \beta$  even when  $S$  approaches its maximum plausible value. Similarly, a smaller lower bound  $L$  typically results in a smaller value for  $S_{\text{likely}}$ , thereby shifting the presumed treatment effect later in the trial. This includes a longer early period with overlapping survival between arms, which requires additional sample size to preserve power. In short, a wider interval  $[L, U]$  reflects greater uncertainty about the separation time and consequently necessitates a larger sample size.
3. The selection of the lower and upper bounds  $L$  and  $U$  should be guided by prior clinical knowledge and expert opinion, as both directly influence the maximum required sample size.

Ideally,  $[L, U]$  should be chosen to cover the plausible range of the true separation time with high confidence, while avoiding unnecessary sample size requirements. This finding aligns with Ye & Yu (2019).

## References

- Horiguchi, M., Hassett, M. & Uno, H. (2019), ‘How do the accrual pattern and followup duration affect the hazard ratio estimate when the proportional hazards assumption is violated?’, *Journal of Biopharmaceutical Statistics* **24**, 867–871.
- Liu, S., Takeda, K. & Rong, A. (2025), ‘Informative event rate in study determination, study design, and interim analysis monitoring with non-proportional hazards’, *Journal of Biopharmaceutical Statistics* .
- Ye, T. & Yu, M. (2019), ‘A robust approach to sample size calculation in cancer immunotherapy trials with delayed treatment effect’, *Biometrics* **75**, 255–266.

Table 5: Percentage of rejecting the null (PRN), percentage of early termination (PET), the actual sample size (each arm), and trial duration under the DTE-BOP2 design with best-guessed separation timepoint  $S_{\text{likely}} = 2, 2.1, 2.2, 2.3, 2.4, 2.5$ , assuming true separation time  $S = 2, 2.5$ , and sample size (28,40) per arm.

| $S_{\text{likely}}$ | S   | True Scenario | PRN (%) | PET (%) | Sample Size | Trial Duration <sup>a</sup> |
|---------------------|-----|---------------|---------|---------|-------------|-----------------------------|
| 2.0                 | 2.0 | $H_0$ holds   | 8.3     | 28.5    | 36.6        | 10.4                        |
|                     |     | $H_1$ holds   | 74.2    | 10.1    | 38.8        | 11.9                        |
|                     | 2.5 | $H_0$ holds   | 8.3     | 23.9    | 37.1        | 10.8                        |
|                     |     | $H_1$ holds   | 71.4    | 9.8     | 38.8        | 11.9                        |
| 2.1                 | 2.0 | $H_0$ holds   | 8.4     | 27.8    | 36.7        | 10.5                        |
|                     |     | $H_1$ holds   | 79.3    | 9.2     | 38.9        | 12.0                        |
|                     | 2.5 | $H_0$ holds   | 8.3     | 23.9    | 37.1        | 10.8                        |
|                     |     | $H_1$ holds   | 76.5    | 8.9     | 38.9        | 12.0                        |
| 2.2                 | 2.0 | $H_0$ holds   | 8.4     | 26.8    | 36.8        | 10.6                        |
|                     |     | $H_1$ holds   | 84.6    | 7.9     | 39.1        | 12.1                        |
|                     | 2.5 | $H_0$ holds   | 8.3     | 23.9    | 37.1        | 10.8                        |
|                     |     | $H_1$ holds   | 81.8    | 8.0     | 39.0        | 12.0                        |
| 2.3                 | 2.0 | $H_0$ holds   | 8.2     | 26.1    | 36.9        | 10.6                        |
|                     |     | $H_1$ holds   | 89.4    | 6.7     | 39.2        | 12.2                        |
|                     | 2.5 | $H_0$ holds   | 8.3     | 23.9    | 37.1        | 10.8                        |
|                     |     | $H_1$ holds   | 87.1    | 7.0     | 39.2        | 12.1                        |
| 2.4                 | 2.0 | $H_0$ holds   | 8.3     | 25.1    | 37.0        | 10.7                        |
|                     |     | $H_1$ holds   | 93.0    | 5.3     | 39.4        | 12.3                        |
|                     | 2.5 | $H_0$ holds   | 8.3     | 23.9    | 37.1        | 10.8                        |
|                     |     | $H_1$ holds   | 91.4    | 6.0     | 39.3        | 12.2                        |
| 2.5                 | 2.0 | $H_0$ holds   | 8.3     | 23.9    | 37.1        | 10.8                        |
|                     |     | $H_1$ holds   | 93.0    | 5.3     | 39.4        | 12.3                        |
|                     | 2.5 | $H_0$ holds   | 8.3     | 23.9    | 37.1        | 10.8                        |
|                     |     | $H_1$ holds   | 91.4    | 6.0     | 39.3        | 12.2                        |

<sup>a</sup> In months.

Table 6: Percentage of rejecting the null (PRN), percentage of early termination (PET), the actual sample size (each arm), and trial duration under the DTE-BOP2 design with sample size (44, 63) per arm across  $S_{\text{likely}}$ .

| Scenario                   |           |       | PRN(%) | PET(%) | Average Sample Size | Duration <sup>a</sup> |
|----------------------------|-----------|-------|--------|--------|---------------------|-----------------------|
| $S_{\text{likely}} = 2$    | $S = 2$   | $H_0$ | 7.8    | 41.8   | 55.1                | 12.7                  |
|                            |           | $H_1$ | 89.1   | 5.5    | 61.9                | 16.0                  |
|                            | $S = 2.1$ | $H_0$ | 8.1    | 41     | 55.2                | 12.8                  |
|                            |           | $H_1$ | 88.3   | 5.9    | 61.9                | 16.0                  |
|                            | $S = 2.2$ | $H_0$ | 8.3    | 41     | 55.3                | 12.8                  |
|                            |           | $H_1$ | 88.3   | 6.1    | 61.8                | 15.9                  |
|                            | $S = 2.3$ | $H_0$ | 8.3    | 39.8   | 55.4                | 12.9                  |
|                            |           | $H_1$ | 87.6   | 6.2    | 61.8                | 15.9                  |
|                            | $S = 2.4$ | $H_0$ | 8.0    | 39.2   | 55.6                | 12.9                  |
|                            |           | $H_1$ | 87.3   | 6.1    | 61.8                | 15.9                  |
|                            | $S = 2.5$ | $H_0$ | 8.2    | 38.4   | 55.7                | 13.0                  |
|                            |           | $H_1$ | 86.9   | 6.2    | 61.8                | 15.9                  |
| $S_{\text{likely}} = 2.25$ | $S = 2$   | $H_0$ | 7.8    | 41.8   | 55.1                | 12.7                  |
|                            |           | $H_1$ | 96.4   | 2.7    | 62.5                | 16.3                  |
|                            | $S = 2.1$ | $H_0$ | 8.1    | 41     | 55.2                | 12.8                  |
|                            |           | $H_1$ | 96.2   | 2.7    | 62.5                | 16.3                  |
|                            | $S = 2.2$ | $H_0$ | 8.3    | 41     | 55.3                | 12.8                  |
|                            |           | $H_1$ | 96.0   | 2.9    | 62.4                | 16.2                  |
|                            | $S = 2.3$ | $H_0$ | 8.3    | 39.8   | 55.4                | 12.9                  |
|                            |           | $H_1$ | 95.9   | 2.8    | 62.5                | 16.2                  |
|                            | $S = 2.4$ | $H_0$ | 8.0    | 39.2   | 55.6                | 12.9                  |
|                            |           | $H_1$ | 95.5   | 3.1    | 62.4                | 16.2                  |
|                            | $S = 2.5$ | $H_0$ | 8.2    | 38.4   | 55.7                | 13.0                  |
|                            |           | $H_1$ | 95.3   | 3.3    | 62.4                | 16.2                  |
| $S_{\text{likely}} = 2.5$  | $S = 2$   | $H_0$ | 7.8    | 41.8   | 55.1                | 12.7                  |
|                            |           | $H_1$ | 99.5   | 0.5    | 62.9                | 16.4                  |
|                            | $S = 2.1$ | $H_0$ | 8.1    | 41     | 55.2                | 12.8                  |
|                            |           | $H_1$ | 99.6   | 0.4    | 62.9                | 16.5                  |
|                            | $S = 2.2$ | $H_0$ | 8.3    | 41     | 55.3                | 12.8                  |
|                            |           | $H_1$ | 99.5   | 0.5    | 62.9                | 16.4                  |
|                            | $S = 2.3$ | $H_0$ | 8.3    | 39.8   | 55.4                | 12.9                  |
|                            |           | $H_1$ | 99.3   | 0.7    | 62.9                | 16.4                  |
|                            | $S = 2.4$ | $H_0$ | 8.0    | 39.2   | 55.6                | 12.9                  |
|                            |           | $H_1$ | 99.1   | 0.9    | 62.8                | 16.4                  |
|                            | $S = 2.5$ | $H_0$ | 8.2    | 38.4   | 55.7                | 13.0                  |
|                            |           | $H_1$ | 99.1   | 0.9    | 62.8                | 16.4                  |

<sup>a</sup> In months.
